# Supplementary material for: G3DR: Generative 3D Reconstruction in ImageNet
Source: arXiv:2403.00939 source file (2024-04-03)
Supplement: Supplementary file 1 [file 07_supp.tex]

% https://drive.google.com/file/d/1Bg5k3IYquph-cZbWJVW0A4kyyd-t7n-d/view?usp=drive_link
\section*{}
%In this supplementary, we submit.
\noindent \update{*Correction*: }After submission, we noticed inconsistencies in the use of variable $i$ in Sec.~3. We apologize for this oversight and will correct the text and equations accordingly in the final paper.

\iffalse
\noindent \update{Update: }After submission, we noticed inconsistencies in the use of variable $i$ in Sec.~3.1 and Sec.~3.2. The updated kernel equation:
\begin{equation}
    k(x, t_i)=max(c_{max}, min(s_1 exp\Biggl(-\frac{(x-t_i)^2}{s_2}\Biggl), c_{min})
  \label{eq:grad_kernel_eq}    
\end{equation}
\noindent where $x$ is the pseudo ground truth depth of the pixel (the distance of the surface from the ray origin). We will correct this and other inconsistencies in the final paper.
\fi

\section{Hyperparameters}
\noindent \textbf{Optimization:} We train $f_{trigen}$ using Adam optimizer with $\beta_1$ = .9; $\beta_2$ = .99, and cosine learning rate schedule with 20K
warmup steps, with an initial learning rate of 2e-6 and a max learning rate of 1e-4. Model $f_{rgbd}$ is trained using a similar setup as LDM3D\cite{stan2023ldm3d}.

\noindent \textbf{Kernel:} Hyperparameters $s_1$ and $s_2$ which control the height and width of the peak of the kernel are set to 1.25 and 0.03 in our experiments. 
Values of $c_{min}$ and $c_{max}$ which determine the maximum and minimum values of the kernel, are set to 0.05 and 1.0.

\noindent \textbf{Losses:} As mentioned in the main paper we $\lambda_1, \lambda_2, \lambda_3, \lambda_4, \lambda_5, \lambda_6$ i.e weights of reconstruction, depth, $vgg$, clip, tv and $vgg_2$ losses are $1$, $2$, $0.5$, $0.35$, $0.1$, $0.5$. We increase $\lambda_4$(clip) from 0.02 to its maximum value of 0.35 linearly over the first 100k steps.
\begin{figure}[t!]
    \centering
    \includegraphics[width=\columnwidth]{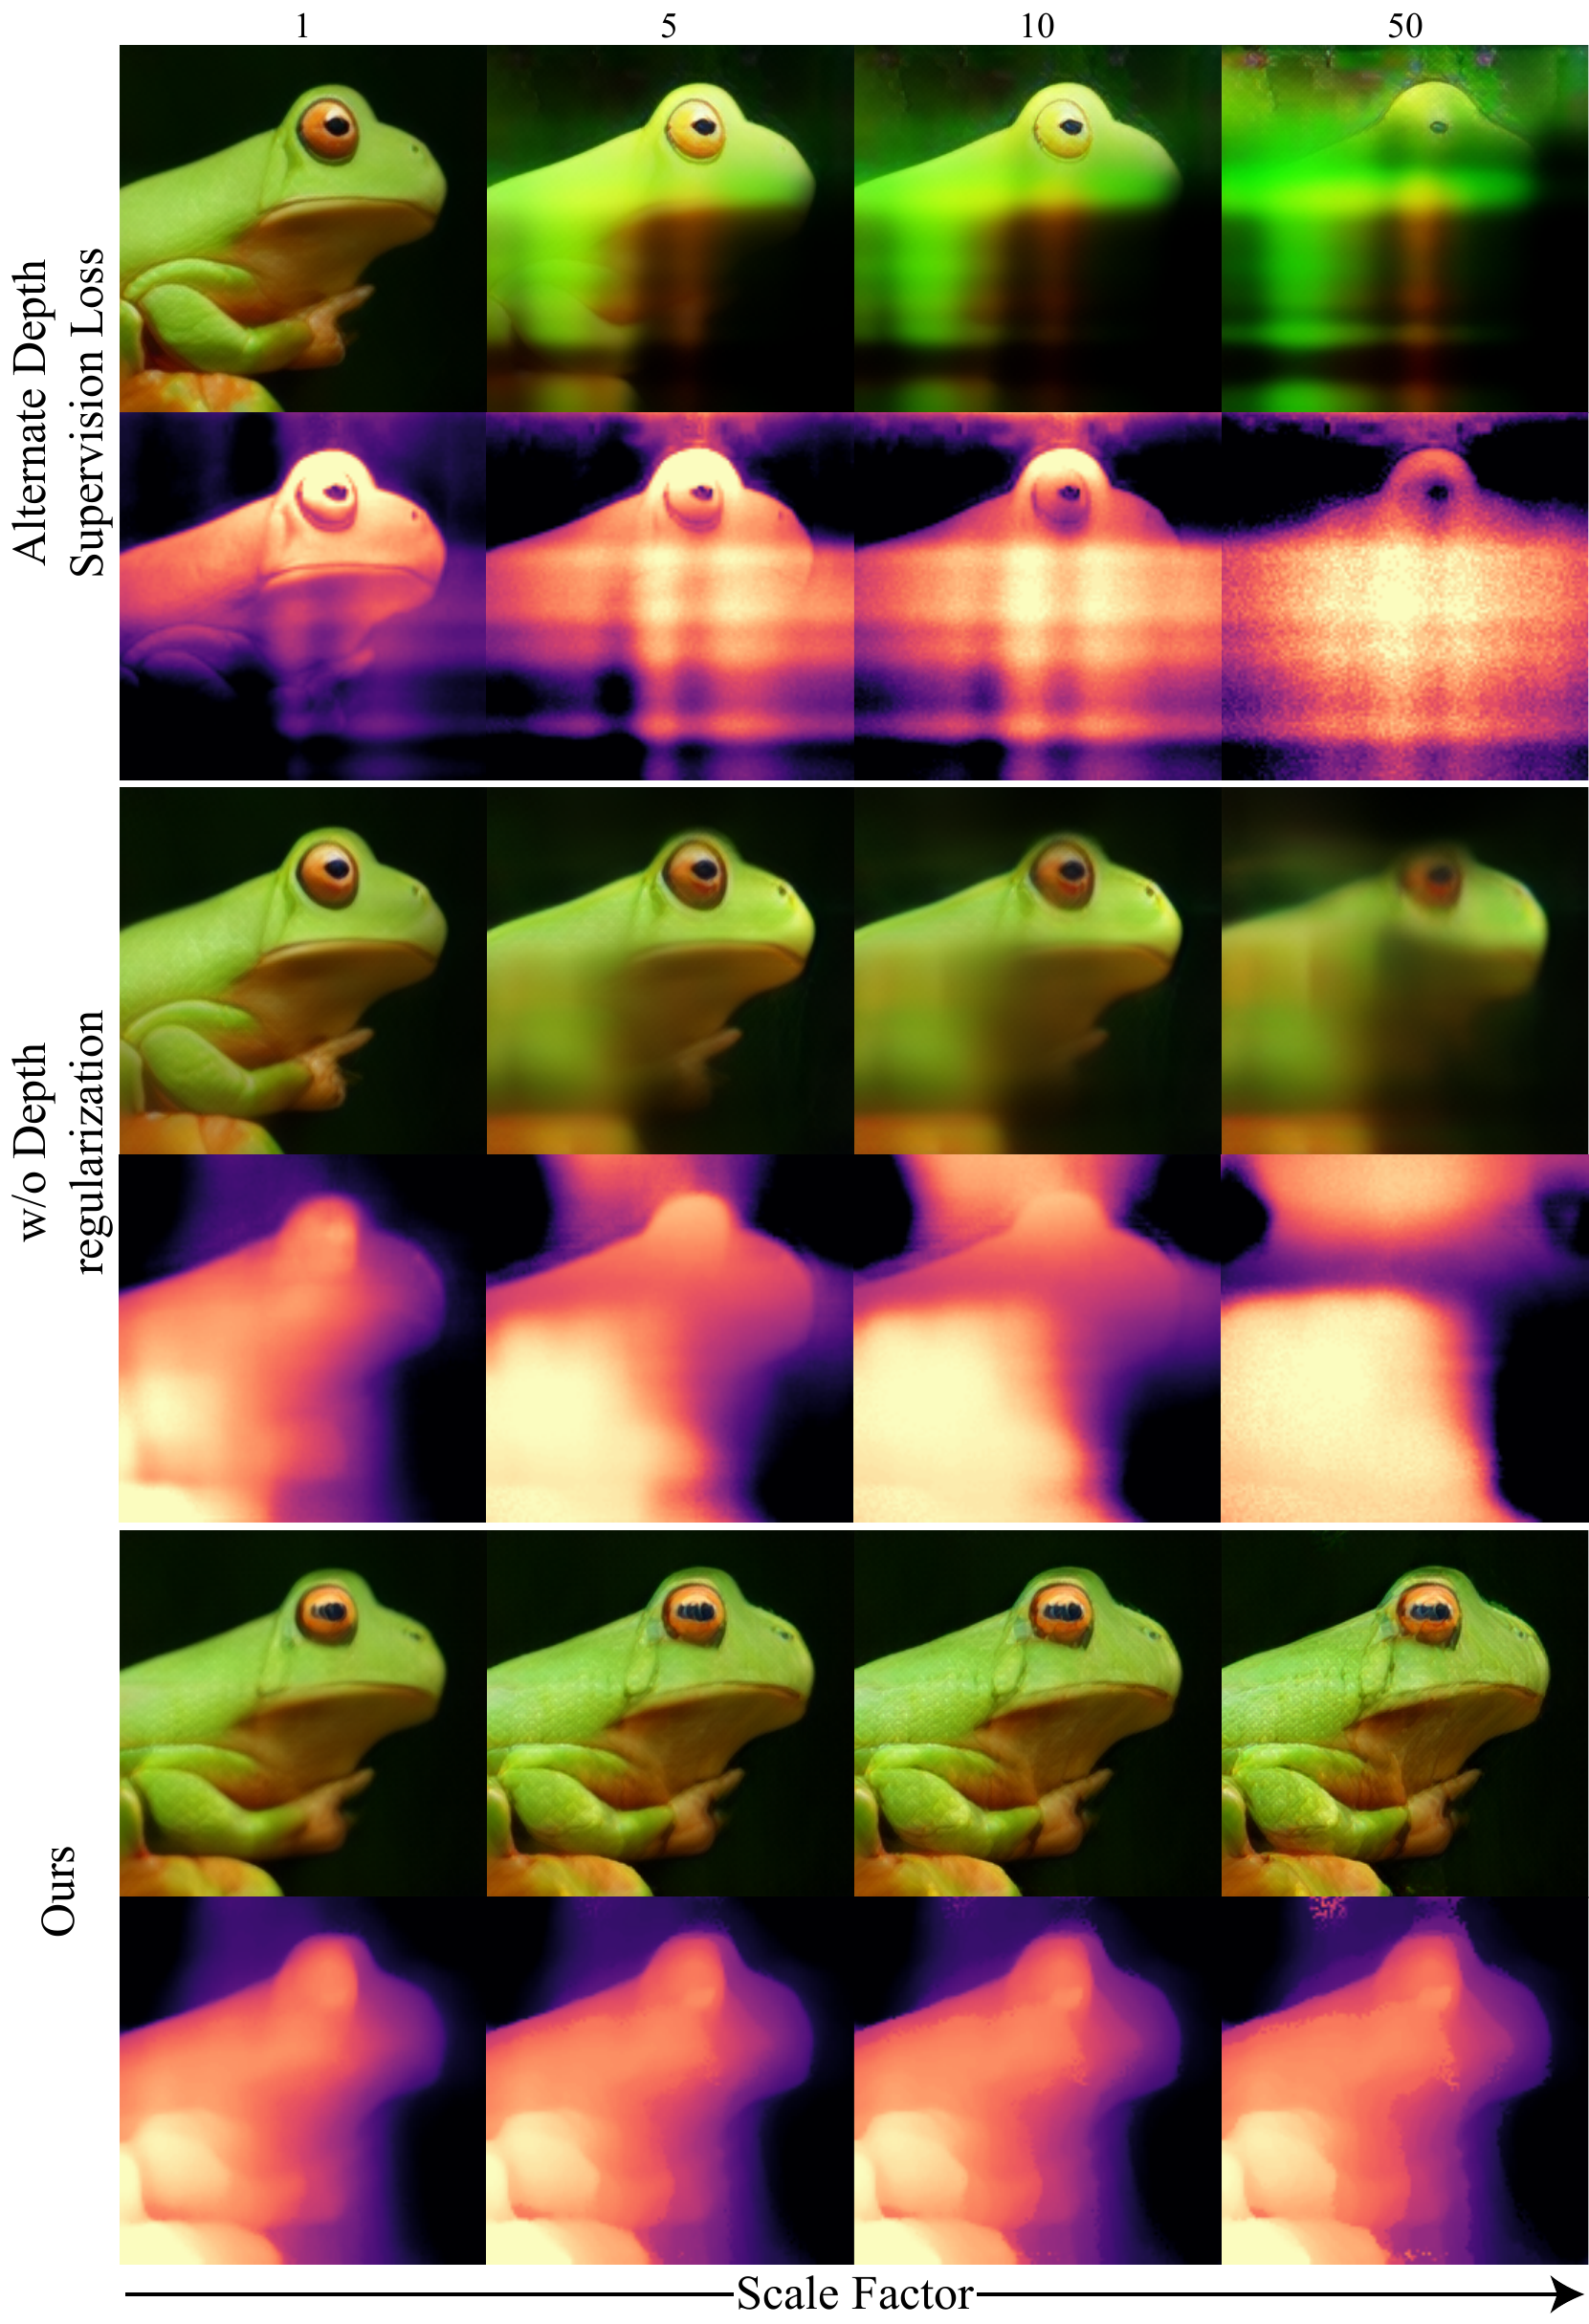}
    \caption{Visualization of $f_{trigen}$ outputs rendered using different scale factors. Notice how the results generated by the model trained using our method degrade gracefully.
    }
    \label{fig:scaling_factor}
    % \vspace{-10pt}
\end{figure}

\section{Alternating between novel and canonical view}
We give more details on how we alternate between the novel and canonical views.
At each iteration, we randomly sample between the canonical and novel views.
We first generate a random number $r$ from a uniform distribution $\mathcal{U}(0,1)$.
Then, we decide if the view is canonical or novel based on the following equation:

\begin{equation}
	\text{view} =
	\begin{cases}
		\text{canon}, & r > min(\tau, 2 \cdot \frac{\text{iter}}{\text{num\_iter}})\\
		\text{novel}, & \text{otherwise.}
	\end{cases}
\label{eq:autolabel}
\end{equation}

\noindent where $\tau$ is a hyperparameter, iter is the current iteration and num\_iter is the total number of iterations.
We set $\tau$ to $0.4$.
Using this procedure, in the early stages of training, we sample mostly canonical views, while sampling very rarely novel views. 
In this way, the main task of the network becomes reconstructing the input image, a much easier task than generating novel views.
In the later stages of training, the probability of sampling novel views linearly increases, until converging at $0.4$.
Thus, the network is tasked to generate novel views, but also to not forget to reconstruct the input image (canon view).

%We randomly sample between the canonical and novel views during training. We design a heuristic probabilistic sampling, where we initially sample with a higher probability for the canonical view. In this way, the network quickly learns the easier task of image reconstruction. We linearly increase the probability of sampling for the novel views during the training, but the probability of sampling a novel view never gets higher than that of sampling the canonical view

\section{Depth regularization geometry ablation}
%\begin{table}[t!]
%\centering
%\begin{tabular}{lllll} 
%\toprule
%Method                            & 1       & 5        & 10       &50    \\ \hline
%Deng et al. 2022           & 26.96   &  27.85  & 26.21     & 22.4   \\ 
%WO Depth Regularization           & 32.58   &  24.91  & 22.34     & 19.38   \\ 
%Ours                              & 31.58   &  31.38  & 31.18     & 30.76  \\ 
%\bottomrule 
%\end{tabular}
%\caption{ablation geo}
%\label{res:ablation_geo}
%\end{table}

\begin{table*}[bth!]
\centering
\begin{tabular}{llllllllll} 
\toprule
  &  \multicolumn{3}{c}{Alternate Depth} & \multicolumn{3}{c}{} & \multicolumn{3}{c}{}\\
  &  \multicolumn{3}{c}{Supervision Loss} & \multicolumn{3}{c}{w/o Depth regularization} & \multicolumn{3}{c}{Ours}\\

Scaling factor  & FID $\downarrow$    & IS $\uparrow$    & NFS $\uparrow$ & FID $\downarrow$    & IS $\uparrow$    & NFS $\uparrow$ & FID $\downarrow$    & IS $\uparrow$    & NFS $\uparrow$         \\ \hline
1         &44.27  &83.04 & 28.96& 13.13 & 116.7& 36.58& 13.12 &151.72 & 36.51\\       
5         &128.64 &12.26 & 29.85& 73.34 & 26.72& 27.97& 12.98 &146.30 & 35.24\\       
10        &174.58 &5.33  & 26.21& 104.91& 14.07& 25.08& 14.42 &131.95 & 35.01\\       
50        &205.15 &3.58  & 22.42& 152.52& 5.94 & 19.38& 21.37 & 99.59 & 34.54\\       
\bottomrule 
\end{tabular}
\caption{Table quantifying the quality of geometry learned by models trained using different methods with various scaling factors.}
\label{res:ablation_geo}
\end{table*}
In Fig. 5 of the main paper, we show color and depth images of models trained with alternative geometric supervision loss, w/o gradient regularization and our pipeline. 
As alternative geometric supervision loss we use the loss function proposed in \cite{kangle2021dsnerf} which supervises the $w$ values using the KL divergence between the $w$ values and depth map. 
In the w/o gradient regularization experiment, we train by supervising the accumulated depth calculated using Eq. 4. 
In both experiments, models result in naive local minima causing volume collapse, we quantify this using the depth accuracy metric in Tab. 4 of the main paper, we further quantify this phenomenon in Tab.~\ref{res:ablation_geo}. 

In Tab. ~\ref{res:ablation_geo} we report FID, IS, NFS metrics for data generated by models trained using different geometric supervision and with different $\sigma$ scaling factors.
The scaling factor augments the predicted $\sigma$ values by multiplication($\sigma_{scaled} = scale factor * \sigma_{predicted}$) before volume rendering.
In the case of networks with volume collapse the generated 3D scenes often incorrectly model surfaces using small $\sigma$ values.
Scaling the $\sigma$ values amplifies these small $\sigma$ values essentially degrading the geometry of predictions with volume collapse.% considerably more compared to predictions with good geometry.
Tab.~\ref{res:ablation_geo} shows how the network trained using our proposed depth regularization degrades gracefully compared to the other methods when increasing the scaling factor. 
This validates that our proposed depth regularization helps a network generate instances with better geometry than the alternatives.
In Fig.~\ref{fig:scaling_factor} we visualize how the color and depth of the renders of outputs from different models change when the scaling factor is increased. 

\section{Multi-resolution sampling}
In Sec. 3.3 of the main paper we mention the multi-resolution triplane sampling strategy we use to improve the generation model performance. The three levels \{$G_1, G_2, G_3$\}we use for sampling have resolution \{128, 64, 32\} respectively. In Fig.~\ref{fig:lod_suppl} we show a visualization of the effect of sampling from only the coarsest level to adding samples from finer levels. 
\begin{figure}[t!]
    \centering
    \includegraphics[width=\columnwidth]{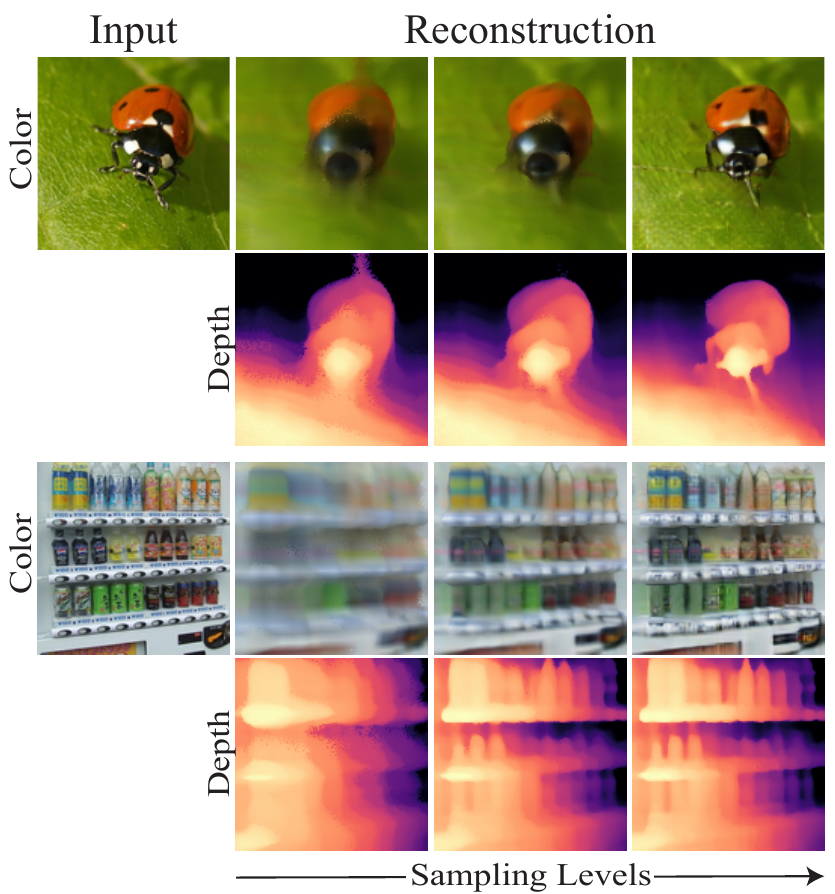}
    \caption{
    Images showing the effect of sampling from different levels. Left to right the images are sampled from  \{$G_3, G_3, G_3$\},  \{$G_2, G_2, G_3$\} and  \{$G_1, G_2, G_3$\}.
    }
    \label{fig:lod_suppl}
    % \vspace{-10pt}
\end{figure}

\section{Evaluation metrics}
\noindent \textbf{Depth accuracy:} We calculate depth accuracy similar to \cite{shi2021lifting}. It is defined as the MSE between rendered and pseudo-ground truth depth normalized using their respective mean and standard deviation.

In the main paper, we do not report the depth accuracy of VQ3D~\cite{DBLP:journals/corr/abs-2302-06833} since they normalize the predicted values using variance. This makes the final metric sensitive to their specific preprocessing and training hyperparameter setup. We will update Tab. 2 of the main paper when the code for VQ3D is available publically.

\noindent \textbf{Non-flatness score:} We adopt the NFS metric from 3DGP\cite{DBLP:conf/iclr/SkorokhodovSXRL23} to quantify the flatness of a generator. We calculate NFS score using the eq:
\begin{equation}
  \begin{array}{l}
    % \mathlarger{w_i = -(1 - exp(-\sigma_i \delta_i)) \ exp\Biggl(\sum\limits_{j=1}^{i-1} \sigma_j} \delta_j \Biggl) \\
    \mathlarger{NFS = \dfrac{1}{N} \sum\limits_{i=1}^{N} exp\Biggl[ -\dfrac{1}{h.w} \sum\limits_{j=1}^{B} b(d^i)_j\Biggl]} \\
  \end{array}
\end{equation}
In our experiments, we use N=256 and B=64.

\noindent \textbf{FID and IS:} We compute Fr$\acute{e}$chet Inception Distance(FID)\cite{heusel2017gans} using similar protocol as Eg3D\cite{DBLP:conf/cvpr/ChanLCNPMGGTKKW22} Inception score(IS) is calculated similarly using \cite{salimans2016improved}.

In Tab.~\ref{res:recon_metric} we present all the evaluation metrics of novel view generation when using ImageNet images with $f_{trigen}$ rather than the images generated using $f_{rgbd}$ like in the main paper.
\begin{table}[ht]
\centering
\resizebox{0.32\textwidth}{!}{
\begin{tabular}{lllll}
\toprule
& FID $\downarrow$    & IS $\uparrow$ & NFS $\uparrow$  & DA $\uparrow$ \\ \hline
Ours& \textbf{11.25}    &  \textbf{168.6}&  \textbf{36.7} &  \textbf{0.33}    \\ 
\bottomrule 
\end{tabular}}
\caption{Quantitative evaluation of novel view generation using images from ImageNet dataset.}
\label{res:recon_metric}
\end{table}

\section{Video results}
We include videos of results presented in the main paper and additional results. All the videos are created using camera parameters with yaw variation of 0.35 and pitch variation of 0.15. In the same folder, we also include the results of our method without the superresolution module in resolution 128x128. We show the same instances in as images in Fig.~\ref{fig:vis1} and Fig.~\ref{fig:vis2}.

\section{Other competing approaches}

Our three main competing approaches are 3DGP, IVID, and VQ3D. We give a brief description of them and the main differences to our method.

\textbf{3DGP \cite{DBLP:conf/iclr/SkorokhodovSXRL23}} (ICLR 2023 Oral) is the first method to tackle the problem of 3D image generation in ImageNet. 
Based on GANs they designed a framework that is able to generate realistically looking 3D objects from the ImageNet dataset.
To do so, they used a depth estimator for geometry preservation and combined it with a flexible camera model, and a knowledge distillation module.
They first sample camera parameters from a prior distribution and pass them to the camera generator.
After that, they use the posterior camera parameters to render an image and its depth map, while using a depth adaptor to bridge the distribution gap between the rendered and the predicted depth.
They also use an image discriminator that receives a 4-channel color-depth image, with the fake sample being color images and their adapted depth map, while the real images are Imagenet images and their estimated depth
In contrast to 3DGP, our method does not use any adversarial training, knowledge distillation module, or depth adapter.

\textbf{IVID \cite{DBLP:journals/corr/abs-2303-17905}} (ICCV 2023) uses a class-condition diffusion model to generate images. 
They do a forward-backward warping of rgbd images, and using another diffusion process they visually complete the images getting in process their novel-view supervision.
To further improve the results, they add blur and texture erosion augmentation.
During inference, they design an autoregressive process to generate the novel views, where each view is conditioned in the previous novel view.
In contrast to IVID, we do not use any warping, blurring, erosion, or autoregressive processes. Their process is also prone to not estimating 3D consistent novel views.

\textbf{VQ3D \cite{DBLP:journals/corr/abs-2302-06833}} (ICCV 2023 oral and honorable mention paper) proposes a 2-stage framework. In the first stage, they learn a model that maps images into a sequence of discrete indices that correspond to a learned latent codebook.
To do so, they design several losses that ensure a good reconstructed canonical view, reasonable novel views, and correct geometry.
Similar to 3DGP, the training process is done in an adversarial manner.
Then in the second stage, they learn an autoregressive model over the discrete encodings produced by Stage 1
encoder, that is able to generate new 3D scenes.
In contrast to them, our method does not use any adversarial training, quantized autoencoder or autoregressive modeling.

As we showed in the experimental section of the main paper, our method despite having a more simple architecture significantly outperforms the three main competing approaches in both visual quality (FID and IS) and geometry (NFS and Depth accuracy).

% \subsection{Limitations}

\begin{figure}[t!]
    \centering
    \includegraphics[width=0.7\columnwidth]{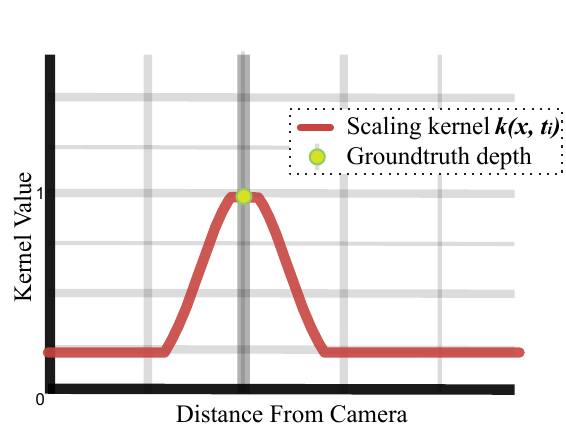}
    \caption{
    An illustration of our kernel shown in 1D.
    }
    \label{fig:1d_illus}
    % \vspace{-10pt}
\end{figure}
\begin{figure*}[t!]
    \centering
    \includegraphics[width=0.85\textwidth]{figures/images/extra_results_imagenet_1.pdf}
    \caption{
    Visualization of results of the results provided along with the supplementary.
    }
    \label{fig:vis1}
    % \vspace{-10pt}
\end{figure*}
\begin{figure*}[t!]
    \centering
    \includegraphics[width=0.85\textwidth]{figures/images/extra_results_imagenet_2.pdf}
    \caption{
    Visualization of results of the results provided along with the supplementary.
    }
    \label{fig:vis2}
    % \vspace{-10pt}
\end{figure*}

\section{1d visual}
We show a 1D illustration of the kernel in Fig.~\ref{fig:1d_illus}. The x-axis represents the distance of the sampled point along the ray from the camera, y-axis represents the magnitude of the kernel.

\section{Code}
We include a development version of our code in the supplemental folder to help the reader reproduce our results. The code is a barebones version created with readability in mind. Many/all important functions are copied to the train.py file for quick perusal and easy reproduction. \textbf{Pre-trained model weights} are available in the links available in the README.md file.

% \subsection{Depth accuracy reporting}

%\subsection{More images (optional) + mentioning videos}

\section*{Broader Impact}

G3DR and stronger models based on it can be used for a variety of applications, including:

\begin{itemize}
\item 3D modeling: G3DR can be used to generate 3D models of objects from single images. This can be useful for a variety of applications, such as product design, architectural visualization, and special effects.
%\item Animation: G3DR can be used to generate 3D assets for animation, such as characters, props, and environments. This can help animators to create more realistic and visually appealing animations.
\item Video games: G3DR can be used to generate 3D assets for video games, such as characters, weapons, and vehicles. This can help game developers to create more immersive and engaging video games.
\end{itemize}

Unfortunately, G3DR, or more powerful models based on it can be used negatively. One potential concern is that G3DR could be used to create realistic-looking fake images or videos (DeepFakes). This could be used for malicious purposes, such as spreading misinformation or propaganda.
%
%In addition, G3DR could be used to create 3D models of people's faces or bodies without their consent. This could be used for privacy-violating purposes, such as tracking people or creating synthetic identities.
%
The authors do not endorse the usage of G3DR for any malicious purpose, such as deep fakes.
